# Supplementary material for: Model-based Preference Optimization in Abstractive Summarization without Human Feedback
Source: arXiv:2409.18618 source file (2024-10-02)
Supplement: Supplementary file 1 [file appendix_main.tex]

\begin{table*}[t!]
\centering
\resizebox{1\textwidth}{!}{%
% \begin{tabular}{c|l|llllllllllll}
\begin{tabular}{c|clcccccccccccc}
\toprule
\multicolumn{2}{c}{}        &                                   & \multicolumn{2}{c}{AlignScore}                        & \multicolumn{2}{c}{FactCC}                            & \multicolumn{2}{c}{BARTScore\uparrow}                         & \multicolumn{2}{c}{BS-FACT}                           & \multicolumn{2}{c}{ROUGE-L}                           & \multicolumn{2}{c}{BERTScore}                         \\
\multicolumn{1}{c}{Dataset} & \multicolumn{1}{c}{Model}   & \multicolumn{1}{c}{Method}    & \multicolumn{1}{c}{Greedy} & \multicolumn{1}{c}{Beam} & \multicolumn{1}{c}{Greedy} & \multicolumn{1}{c}{Beam} & \multicolumn{1}{c}{Greedy} & \multicolumn{1}{c}{Beam} & \multicolumn{1}{c}{Greedy} & \multicolumn{1}{c}{Beam} & \multicolumn{1}{c}{Greedy} & \multicolumn{1}{c}{Beam} & \multicolumn{1}{c}{Greedy} & \multicolumn{1}{c}{Beam} \\
\arrayrulecolor{black}\midrule

 \multirow{15}{*}{\rotatebox{90}{TL;DR}} & \multirow{6}{*}{GPT-J-6B}   & SFT  & 83.54  & 89.21 &   53.48   &   64.18  & -1.63  & -1.25   &  90.30  &  91.53  &   26.01    &  26.74    &  88.67  & 88.68  \\ &
   & PPO (\textit{w/ human pref.})  & 75.88   &  83.10  &  47.52  &  54.40  &  -1.80     & -1.35 &  89.78  &  91.32   &   23.28  &  23.55  &  87.87  &  87.68  \\ &

& DPO (\textit{w/ human pref.}) &   82.55  &  88.12  &   54.09  &  61.70 &  -1.65   &  -1.33   &   90.22  &  91.27   &  26.28 &  \textbf{27.24}  &  \textbf{88.84}  & \textbf{88.85}  \\
\arrayrulecolor{black}\cmidrule{3-15}
& & ProPO (\textit{Iteration 1})   &   86.82  &  91.61   &  59.39  & 72.10  & -1.41  &  -1.10  &  91.20   &   92.20  &  \textbf{26.49}  &  26.10   &  88.80  &  88.50 \\ &
 & ProPO (\textit{Iteration 2}) &  88.14 &  93.34 & 62.02  & 76.45  & -1.29  & -0.99  &  91.61  &  92.57  &  26.03   &  25.28  & 88.60   & 88.18 \\ &
& ProPO (\textit{Iteration 3}) & \textbf{93.80}  &  \textbf{95.31} &  \textbf{76.18}  & \textbf{82.62}  & \textbf{-1.01} & \textbf{-0.98} &  \textbf{92.72}  &  \textbf{92.73}  &  24.79   &  24.21  &  88.07  & 87.89 \\
\arrayrulecolor{black}\cmidrule{2-15}                           
& \multirow{4}{*}{Mistral-7B} & SFT  &  82.74  &   87.85  &    24.72   &   41.87    &  -1.81  &   -1.48  & 90.04 &  90.96  &  \textbf{25.02}  &  \textbf{25.32}   & \textbf{88.44} &  \textbf{88.36} \\
\arrayrulecolor{black}\cmidrule{3-15}
% \midrule
& & ProPO (\textit{Iteration 1})  &  88.44   &   92.78  &   36.96 &   57.32   &   -1.50  &  -1.23  &  91.28  &   91.99 & 24.51  & 23.85 &   88.29  &  88.01 \\
 & & ProPO (\textit{Iteration 2}) &  \textbf{93.55} &   \textbf{96.28}  &  69.24   &  84.33   &   \textbf{-1.05}   &  -0.93 &  \textbf{92.57}   &  92.86   &  23.12  &  22.09  &  87.43   & 87.20  \\
 &  & ProPO (\textit{Iteration 3}) & 84.85  &  94.21 & \textbf{79.29}  & \textbf{92.69}  & -1.27  &  \textbf{-0.87} &  92.41   & \textbf{93.08}  &   21.34  & 21.78 & 85.97  &  86.58 \\
\arrayrulecolor{black}\cmidrule{2-15}                        
& \multirow{4}{*}{LLaMA2-7B} & SFT    &  77.68  &  84.92   &    23.36   &   29.06   & -2.05   & -1.65 & 89.56 &  90.58 &  \textbf{23.33}  &  \textbf{24.31} & \textbf{88.31} & \textbf{88.37} \\
\arrayrulecolor{black}\cmidrule{3-15}
& & ProPO (\textit{Iteration 1})   &   78.28  &  \textbf{85.30}   &  \textbf{23.44}  &   \textbf{29.31}   &  -2.03   &  -1.64  &  89.64  &  90.66  &  23.20 & 24.22 &  88.26  &  88.33 \\
& & ProPO (\textit{Iteration 2}) & \textbf{78.38}  &   85.16  &  23.07   &   28.83  &   \textbf{-2.03}   &  \textbf{-1.64} &  \textbf{89.68}   &   \textbf{90.67}  &  23.15  &  24.12  &   88.26  &  88.30 \\
 &  &  ProPO (\textit{Iteration 3}) &    78.07    &  84.83 &  22.14 &    28.19  & -2.05  & -1.66  &  89.61   & 90.59  &  23.09   & 24.04 &  88.26 & 88.31 \\
\arrayrulecolor{black}\midrule   

\multirow{9}{*}{\rotatebox{90}{XSUM}} & \multirow{4}{*}{Mistral-7B} & SFT  &  60.00  & 66.31   &   23.65   &     25.92  &  -1.97 &  -1.96   & 89.19 &  89.15  &  \textbf{31.16}  &  30.65   & \textbf{90.51} &  89.98 \\
\arrayrulecolor{black}\cmidrule{3-15}
& & ProPO (\textit{Iteration 1})  &   61.03  & 67.67    & \textbf{23.72}  &   \textbf{27.69}  &  -1.98 &  -2.06 &  89.23 &  89.08 &  30.48 & 28.96 & 90.30   &  89.44 \\
 & & ProPO (\textit{Iteration 2}) & 61.66 &  67.12  & 23.39  &  24.82  & -1.94   & \textbf{-1.83}  & 89.33   & \textbf{89.54}  &  31.12 &  \textbf{30.74}  &  90.48  & \textbf{90.12} \\
 &  & ProPO (\textit{Iteration 3}) & \textbf{63.51} & \textbf{67.86}  & 22.97 &  26.65 & \textbf{-1.92} & -1.90 &  \textbf{89.41}  &  89.50 &  30.80  & 30.37 & 90.36 &  90.11 \\
 
\arrayrulecolor{black}\cmidrule{2-15}            & \multirow{4}{*}{LLaMA2-7B} & SFT  &  57.57  &  65.80  &   24.40   &   27.50    & -2.06  &  -1.80   & 88.96 &  89.47  &  27.76  &  30.36   & 89.94 &  90.29 \\
\arrayrulecolor{black}\cmidrule{3-15}
& & ProPO (\textit{Iteration 1})  &  58.20   &   66.31  &  24.40 &   27.04  & -2.06  & -1.82  & 88.99  &89.48 & 27.88  & 30.23 &  89.98  & 90.28  \\
 & & ProPO (\textit{Iteration 2}) & 59.24 &  66.12  & 24.46  & 27.07   &   -2.05 & -1.80  & 89.01   & \textbf{89.51}  &  28.06 &  30.20  &  89.98  & 90.28 \\
 &  & ProPO (\textit{Iteration 3}) & \textbf{60.42}  &  \textbf{67.13} & \textbf{25.15} &  \textbf{28.88} & \textbf{-2.03}  & \textbf{-1.80} &  \textbf{89.07}  &  89.50 &  \textbf{28.56}  & \textbf{30.54} & \textbf{90.05} & \textbf{90.32} \\

\arrayrulecolor{black}\bottomrule 
\arrayrulecolor{black}\bottomrule                   
\end{tabular}
}
\caption{Comparison of iterative preference optimization methods with SFT and human preference optimized models. PPO and DPO represent models trained with human-annotated data. Our method, $M_t$, utilizes results by beam search decoding from $M_{t-1}$ as chosen responses and temperature-scaled sampling generations from $M_0$ as rejected responses for preference optimization. The results indicate that the iterative approach enhances summarization outcomes in terms of faithfulness and relevance metrics compared to SFT and human preference optimized methods.
}
\end{table*}
